# Supplementary material for: Complementary Vanishing Graphs
Source: arXiv:2207.07294 source file (2022-07-15)
Supplement: Supplementary file 1 [file appendix.pdf]

# A Complementary vanishing graphs on $n \leq 8$ vertices

| $G$ | $\overline{G}$ | $A$ | $B$ |
|---|---|---|---|
| 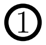 $K_1$ : `@` | 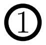 $\overline{K}_1$ : `@` | $\begin{bmatrix}1\end{bmatrix}$ | $\begin{bmatrix}0\end{bmatrix}$ |
| 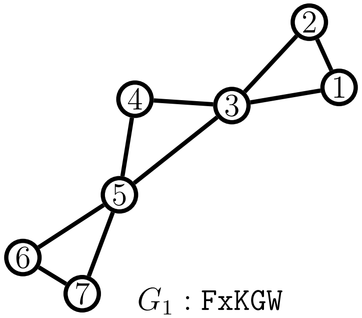 $G_1$ : `FxKGW` | 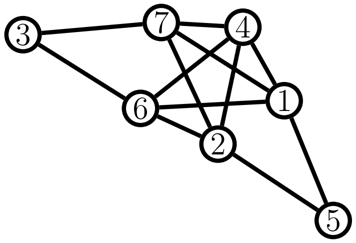 $\overline{G}_1$ : `FErv_` | $\begin{bmatrix}1&1&1&0&0&0&0\\1&1&1&0&0&0&0\\1&1&2&1&-1&0&0\\0&0&1&1&-1&0&0\\0&0&-1&-1&2&1&-1\\0&0&0&0&1&1&-1\\0&0&0&0&-1&-1&1\end{bmatrix}$ | $\begin{bmatrix}0&0&0&2&2&-1&1\\0&0&0&-2&-2&-1&-3\\0&0&0&0&0&2&2\\2&-2&0&0&0&-2&-2\\2&-2&0&0&0&0&0\\-1&-1&2&-2&0&0&0\\1&-3&2&-2&0&0&0\end{bmatrix}$ |
| 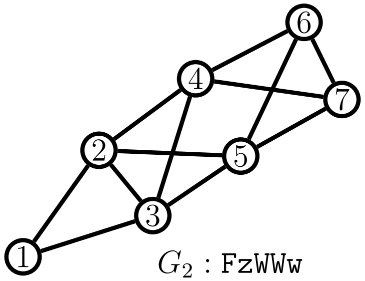 $G_2$ : `FzWWw` | 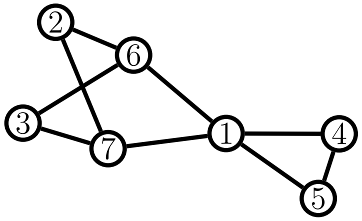 $\overline{G}_2$ : `FCff?` | $\begin{bmatrix}0&1&1&0&0&0&0\\1&3&2&1&-1&0&0\\1&2&1&1&-1&0&0\\0&1&1&0&0&1&1\\0&-1&-1&0&0&1&1\\0&0&0&1&1&1&1\\0&0&0&1&1&1&1\end{bmatrix}$ | $\begin{bmatrix}4&0&0&-2&2&-1&1\\0&0&0&0&0&1&-1\\0&0&0&0&0&-1&1\\-2&0&0&1&-1&0&0\\2&0&0&-1&1&0&0\\-1&1&-1&0&0&0&0\\1&-1&1&0&0&0&0\end{bmatrix}$ |
| 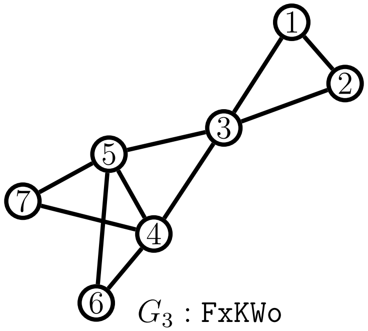 $G_3$ : `FxKWo` | 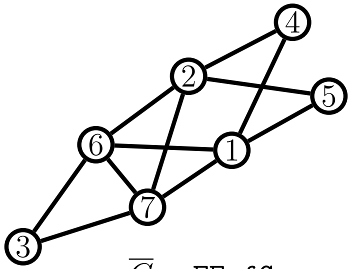 $\overline{G}_3$ : `FErfG` | $\begin{bmatrix}1&1&1&0&0&0&0\\1&1&1&0&0&0&0\\1&1&1&1&-1&0&0\\0&0&1&-1&1&1&1\\0&0&-1&1&-1&-1&-1\\0&0&0&1&-1&0&0\\0&0&0&1&-1&0&0\end{bmatrix}$ | $\begin{bmatrix}0&0&0&2&2&-1&1\\0&0&0&-2&-2&-1&1\\0&0&0&0&0&2&-2\\2&-2&0&0&0&0&0\\2&-2&0&0&0&0&0\\-1&-1&2&0&0&-4&2\\1&1&-2&0&0&2&0\end{bmatrix}$ |

| | | | |
|---|---|---|---|
| 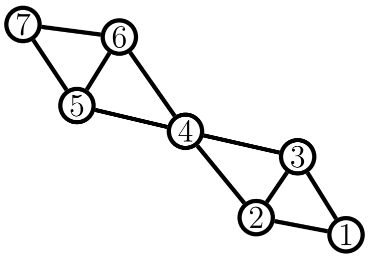 $G_4$ : FzCWW | 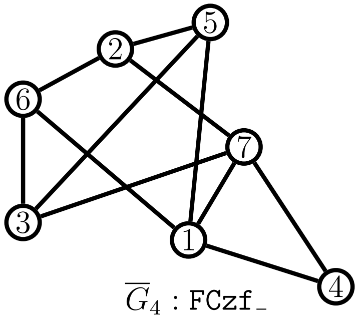 $\overline{G}_4$ : FCzf_ | $\begin{bmatrix} 0 & 2 & 2 & 0 & 0 & 0 & 0 \\ 2 & -1 & 1 & 2 & 0 & 0 & 0 \\ 2 & 1 & 3 & 2 & 0 & 0 & 0 \\ 0 & 2 & 2 & 0 & 2 & -2 & 0 \\ 0 & 0 & 0 & 2 & -1 & -1 & 2 \\ 0 & 0 & 0 & -2 & -1 & 3 & -2 \\ 0 & 0 & 0 & 0 & 2 & -2 & 0 \end{bmatrix}$ | $\begin{bmatrix} 1 & 0 & 0 & -1 & 1 & 1 & 2 \\ 0 & 0 & 0 & 0 & 1 & 1 & 1 \\ 0 & 0 & 0 & 0 & -1 & -1 & -1 \\ -1 & 0 & 0 & 1 & 0 & 0 & 1 \\ 1 & 1 & -1 & 0 & 0 & 0 & 0 \\ 1 & 1 & -1 & 0 & 0 & 0 & 0 \\ 2 & 1 & -1 & -1 & 0 & 0 & 1 \end{bmatrix}$ |
| 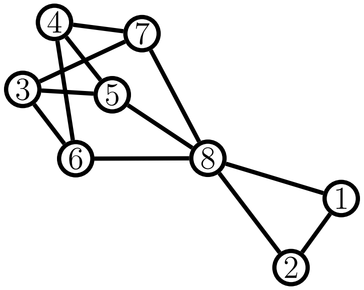 $G_5$ : G_Kpe[ | 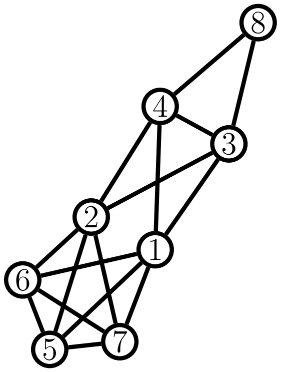 $\overline{G}_5$ : G^rMX_ | $\begin{bmatrix} 1 & 1 & 0 & 0 & 0 & 0 & 0 & -1 \\ 1 & 1 & 0 & 0 & 0 & 0 & 0 & -1 \\ 0 & 0 & 0 & 0 & -2 & -2 & -1 & 0 \\ 0 & 0 & 0 & 0 & 2 & 2 & 1 & 0 \\ 0 & 0 & -2 & 2 & 0 & 0 & 0 & 2 \\ 0 & 0 & -2 & 2 & 0 & 0 & 0 & 2 \\ 0 & 0 & -1 & 1 & 0 & 0 & 0 & 1 \\ -1 & -1 & 0 & 0 & 2 & 2 & 1 & 1 \end{bmatrix}$ | $\begin{bmatrix} 0 & 0 & 8 & 8 & -4 & 2 & 4 & 0 \\ 0 & 0 & -5 & -5 & 4 & -2 & -4 & 0 \\ 8 & -5 & 0 & -3 & 0 & 0 & 0 & 3 \\ 8 & -5 & -3 & -6 & 0 & 0 & 0 & 3 \\ -4 & 4 & 0 & 0 & 3.5 & -2 & -3 & 0 \\ 2 & -2 & 0 & 0 & -2 & 0 & 4 & 0 \\ 4 & -4 & 0 & 0 & -3 & 4 & -2 & 0 \\ 0 & 0 & 3 & 3 & 0 & 0 & 0 & 0 \end{bmatrix}$ |
| 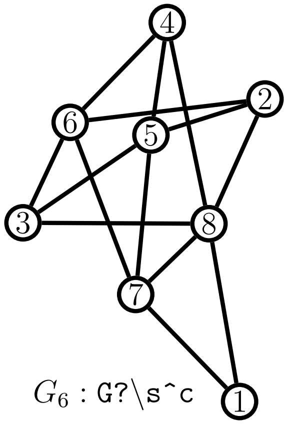 $G_6$ : G?\s^c | 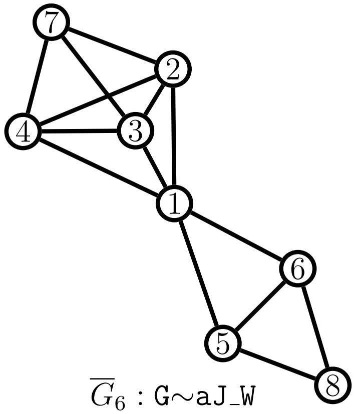 $\overline{G}_6$ : G∼aJ_W | $\begin{bmatrix} -7 & 0 & 0 & 0 & 0 & 0 & -7 & 7 \\ 0 & 0 & 0 & 0 & -3 & -6 & 0 & 6 \\ 0 & 0 & 0 & 0 & 1 & 2 & 0 & -2 \\ 0 & 0 & 0 & 0 & 2 & 4 & 0 & -4 \\ 0 & -3 & 1 & 2 & 0 & 0 & 1 & 0 \\ 0 & -6 & 2 & 4 & 0 & 0 & 2 & 0 \\ -7 & 0 & 0 & 0 & 1 & 2 & -7 & 5 \\ 7 & 6 & -2 & -4 & 0 & 0 & 5 & -7 \end{bmatrix}$ | $\begin{bmatrix} 0 & 1 & -1 & 2 & -2 & 1 & 0 & 0 \\ 1 & -2 & -1 & -2 & 0 & 0 & -1 & 0 \\ -1 & -1 & 0 & -2 & 0 & 0 & 1 & 0 \\ 2 & -2 & -2 & -1 & 0 & 0 & -2 & 0 \\ -2 & 0 & 0 & 0 & 0 & -2 & 0 & -2 \\ 1 & 0 & 0 & 0 & -2 & 2 & 0 & 1 \\ 0 & -1 & 1 & -2 & 0 & 0 & 0 & 0 \\ 0 & 0 & 0 & 0 & -2 & 1 & 0 & 0 \end{bmatrix}$ |

<table>
<tr>
<td>
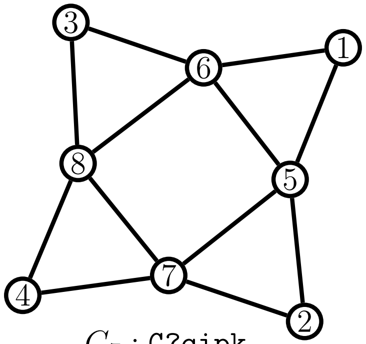


$G_7$ : G?qipk
</td>
<td>
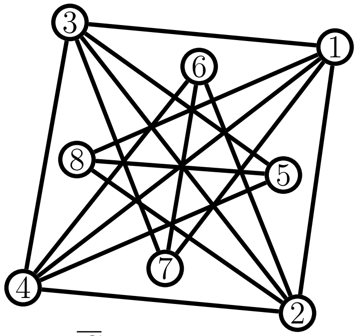


$\overline{G}_7$ : G~LTMO
</td>
<td>

$$\begin{bmatrix} 6 & 0 & 0 & 0 & 6 & 3 & 0 & 0 \\ 0 & -8 & 0 & 0 & 4 & 0 & 8 & 0 \\ 0 & 0 & -2 & 0 & 0 & -1 & 0 & -2 \\ 0 & 0 & 0 & 3 & 0 & 0 & -3 & 3 \\ 6 & 4 & 0 & 0 & 4 & 3 & -4 & 0 \\ 3 & 0 & -1 & 0 & 3 & 1 & 0 & -1 \\ 0 & 8 & 0 & -3 & -4 & 0 & -5 & -3 \\ 0 & 0 & -2 & 3 & 0 & -1 & -3 & 1 \end{bmatrix}$$

</td>
<td>

$$\begin{bmatrix} 0 & -1 & 2 & 1 & 0 & 0 & -1 & -2 \\ -1 & 0 & -2 & -1 & 0 & 2 & 0 & 1 \\ 2 & -2 & 0 & -1 & -2 & 0 & -1 & 0 \\ 1 & -1 & -1 & 0 & -2 & 2 & 0 & 0 \\ 0 & 0 & -2 & -2 & 0 & 0 & 0 & 2 \\ 0 & 2 & 0 & 2 & 0 & 0 & 2 & 0 \\ -1 & 0 & -1 & 0 & 0 & 2 & 0 & 0 \\ -2 & 1 & 0 & 0 & 2 & 0 & 0 & 0 \end{bmatrix}$$

</td>
</tr>
<tr>
<td>
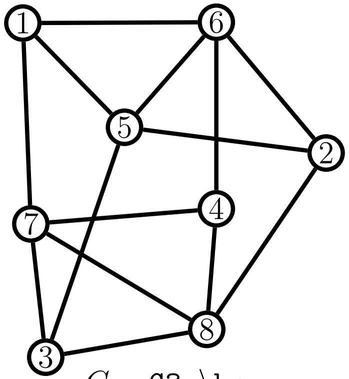


$G_8$ : G?z\bc
</td>
<td>
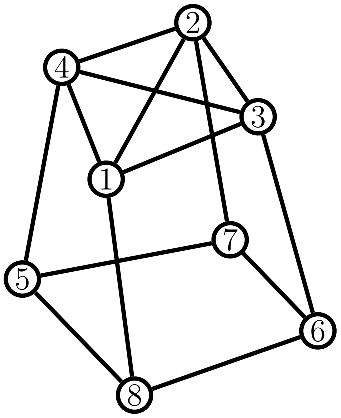


$\overline{G}_8$ : G~Ca[W
</td>
<td>

$$\begin{bmatrix} 8 & 0 & 0 & 0 & 8 & 4 & -4 & 0 \\ 0 & 8 & 0 & 0 & 8 & 4 & 0 & 4 \\ 0 & 0 & -4 & 0 & -8 & 0 & 2 & -2 \\ 0 & 0 & 0 & -1 & 0 & -2 & 1 & -1 \\ 8 & 8 & -8 & 0 & 0 & 8 & 0 & 0 \\ 4 & 4 & 0 & -2 & 8 & 0 & 0 & 0 \\ -4 & 0 & 2 & 1 & 0 & 0 & 0 & 2 \\ 0 & 4 & -2 & -1 & 0 & 0 & 2 & 0 \end{bmatrix}$$

</td>
<td>

$$\begin{bmatrix} 0 & -2 & -2 & -4 & 0 & 0 & 0 & 4 \\ -2 & 0 & -2 & -4 & 0 & 0 & -4 & 0 \\ -2 & -2 & 0 & -8 & 0 & 4 & 0 & 0 \\ -4 & -4 & -8 & 0 & 4 & 0 & 0 & 0 \\ 0 & 0 & 0 & 4 & 1 & 0 & 2 & -2 \\ 0 & 0 & 4 & 0 & 0 & 4 & 4 & -4 \\ 0 & -4 & 0 & 0 & 2 & 4 & 8 & 0 \\ 4 & 0 & 0 & 0 & -2 & -4 & 0 & 8 \end{bmatrix}$$

</td>
</tr>
<tr>
<td>
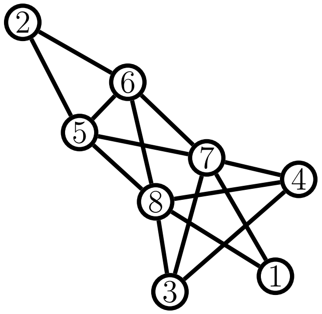


$G_9$ : G@PL|w
</td>
<td>
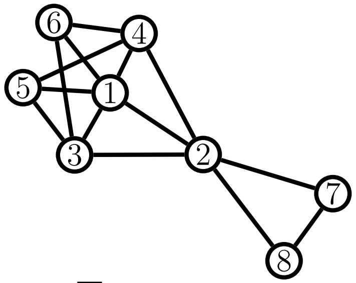


$\overline{G}_9$ : G}mqAC
</td>
<td>

$$\begin{bmatrix} 0 & 0 & 0 & 0 & 0 & 0 & -2 & -2 \\ 0 & 0 & 0 & 0 & 1 & -1 & 0 & 0 \\ 0 & 0 & 2 & 2 & 0 & 0 & -2 & -2 \\ 0 & 0 & 2 & 2 & 0 & 0 & 1 & 1 \\ 0 & 1 & 0 & 0 & 0 & 1 & -2 & 1 \\ 0 & -1 & 0 & 0 & 1 & -2 & 1 & -2 \\ -2 & 0 & -2 & 1 & -2 & 1 & 0 & 0 \\ -2 & 0 & -2 & 1 & 1 & -2 & 0 & 0 \end{bmatrix}$$

</td>
<td>

$$\begin{bmatrix} 3 & 3 & -1 & 1 & -3 & -3 & 0 & 0 \\ 3 & 36 & -2 & 2 & 0 & 0 & 12 & -12 \\ -1 & -2 & 0 & 0 & 2 & 2 & 0 & 0 \\ 1 & 2 & 0 & 0 & -2 & -2 & 0 & 0 \\ -3 & 0 & 2 & -2 & 0 & 0 & 0 & 0 \\ -3 & 0 & 2 & -2 & 0 & 0 & 0 & 0 \\ 0 & 12 & 0 & 0 & 0 & 0 & 4 & -4 \\ 0 & -12 & 0 & 0 & 0 & 0 & -4 & 4 \end{bmatrix}$$

</td>
</tr>
</table>

| | | | |
|---|---|---|---|
| 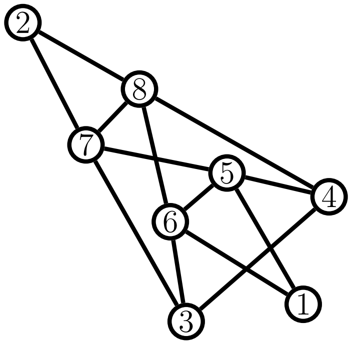 $G_{10}$ : G@ejQk | 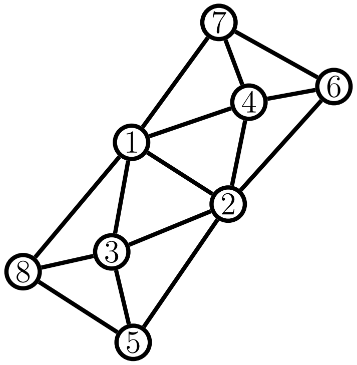 $\overline{G}_{10}$ : G}XSlO | $\begin{bmatrix} -12 & 0 & 0 & 0 & -6 & 12 & 0 & 0 \\ 0 & 8 & 0 & 0 & 0 & 0 & 8 & 8 \\ 0 & 0 & 0 & -4 & 0 & 2 & -4 & 0 \\ 0 & 0 & -4 & 0 & 2 & 0 & 0 & -4 \\ -6 & 0 & 0 & 2 & -3 & 5 & 2 & 0 \\ 12 & 0 & 2 & 0 & 5 & -12 & 0 & 2 \\ 0 & 8 & -4 & 0 & 2 & 0 & 8 & 4 \\ 0 & 8 & 0 & -4 & 0 & 2 & 4 & 8 \end{bmatrix}$ | $\begin{bmatrix} 0 & 1 & -1 & 2 & 0 & 0 & -2 & 1 \\ 1 & 0 & 1 & 1 & 2 & 2 & 0 & 0 \\ -1 & 1 & 2 & 0 & 2 & 0 & 0 & -1 \\ 2 & 1 & 0 & 2 & 0 & 2 & -1 & 0 \\ 0 & 2 & 2 & 0 & 0 & 0 & 0 & -2 \\ 0 & 2 & 0 & 2 & 0 & 0 & -2 & 0 \\ -2 & 0 & 0 & -1 & 0 & -2 & 0 & 0 \\ 1 & 0 & -1 & 0 & -2 & 0 & 0 & 0 \end{bmatrix}$ |
| 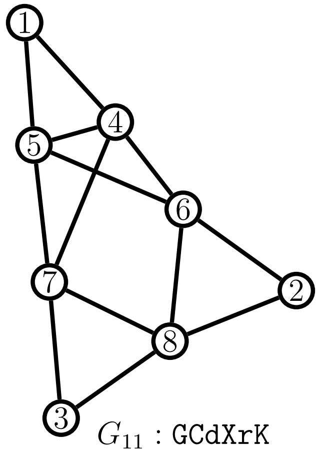 $G_{11}$ : GCdXrK | 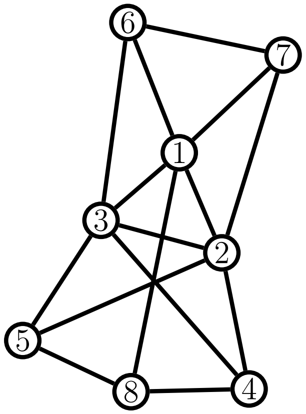 $\overline{G}_{11}$ : GzYeKo | $\begin{bmatrix} 0 & 0 & 0 & -4 & 4 & 0 & 0 & 0 \\ 0 & -2 & 0 & 0 & 0 & -2 & 0 & -4 \\ 0 & 0 & 2 & 0 & 0 & 0 & -2 & 4 \\ -4 & 0 & 0 & -3 & -1 & 4 & -4 & 0 \\ 4 & 0 & 0 & -1 & 5 & -4 & 4 & 0 \\ 0 & -2 & 0 & 4 & -4 & -2 & 0 & -4 \\ 0 & 0 & -2 & -4 & 4 & 0 & 2 & -4 \\ 0 & -4 & 4 & 0 & 0 & -4 & -4 & 0 \end{bmatrix}$ | $\begin{bmatrix} -2 & -1 & -1 & 0 & 0 & -1 & 1 & 1 \\ -1 & 0 & -1 & 2 & 2 & 0 & -1 & 0 \\ -1 & -1 & 0 & 2 & 2 & 1 & 0 & 0 \\ 0 & 2 & 2 & 0 & 0 & 0 & 0 & -1 \\ 0 & 2 & 2 & 0 & 0 & 0 & 0 & -1 \\ -1 & 0 & 1 & 0 & 0 & 0 & 1 & 0 \\ 1 & -1 & 0 & 0 & 0 & 1 & 0 & 0 \\ 1 & 0 & 0 & -1 & -1 & 0 & 0 & 0 \end{bmatrix}$ |
| 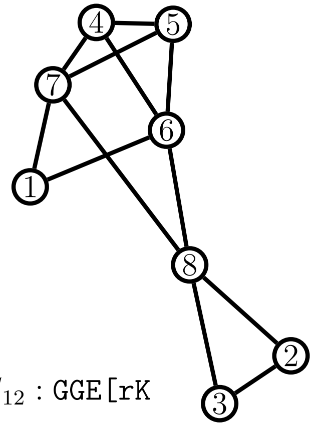 $G_{12}$ : GGE[rK | 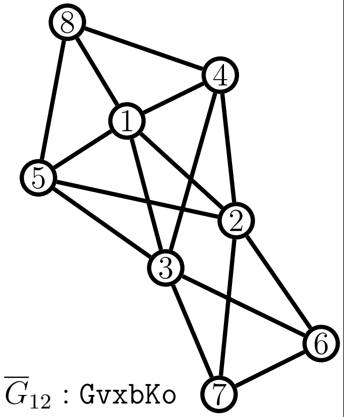 $\overline{G}_{12}$ : GvxbKo | $\begin{bmatrix} 0 & 0 & 0 & -4 & 4 & 0 & 0 & 0 \\ 0 & -2 & 0 & 0 & 0 & -2 & 0 & -4 \\ 0 & 0 & 2 & 0 & 0 & 0 & -2 & 4 \\ -4 & 0 & 0 & -3 & -1 & 4 & -4 & 0 \\ 4 & 0 & 0 & -1 & 5 & -4 & 4 & 0 \\ 0 & -2 & 0 & 4 & -4 & -2 & 0 & -4 \\ 0 & 0 & -2 & -4 & 4 & 0 & 2 & -4 \\ 0 & -4 & 4 & 0 & 0 & -4 & -4 & 0 \end{bmatrix}$ | $\begin{bmatrix} -2 & 1 & -2 & 2 & 2 & 0 & 0 & -1 \\ 1 & 0 & 0 & -2 & -2 & -1 & 1 & 0 \\ -2 & 0 & 0 & 4 & 4 & 1 & -1 & 0 \\ 2 & -2 & 4 & 0 & 0 & 0 & 0 & 2 \\ 2 & -2 & 4 & 0 & 0 & 0 & 0 & 2 \\ 0 & -1 & 1 & 0 & 0 & 3 & -3 & 0 \\ 0 & 1 & -1 & 0 & 0 & -3 & 3 & 0 \\ -1 & 0 & 0 & 2 & 2 & 0 & 0 & 0 \end{bmatrix}$ |

<table>
<tr>
<td>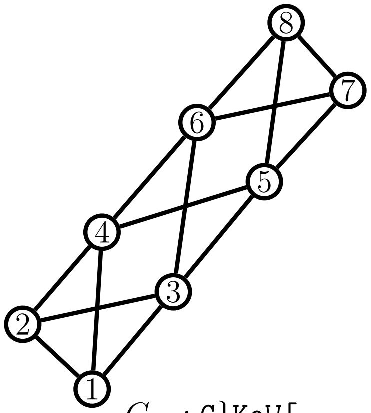<br>$G_{13}$ : G}KoW[</td>
<td>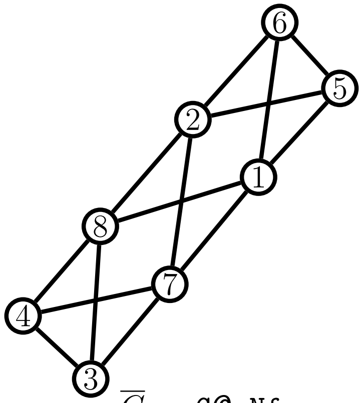<br>$\overline{G}_{13}$ : G@rNf_</td>
<td>$\begin{bmatrix} 1 & 1 & 0 & 0 & 1 & 1 & 0 & 0 \\ 1 & 1 & 0 & 0 & 1 & 1 & 0 & 0 \\ 0 & 0 & 1 & 1 & 0 & 0 & 1 & 1 \\ 0 & 0 & 1 & 1 & 0 & 0 & 1 & 1 \\ 1 & 1 & 0 & 0 & 0 & 0 & 1 & 1 \\ 1 & 1 & 0 & 0 & 0 & 0 & 1 & 1 \\ 0 & 0 & 1 & 1 & 1 & 1 & 0 & 0 \\ 0 & 0 & 1 & 1 & 1 & 1 & 0 & 0 \end{bmatrix}$</td>
<td>$\begin{bmatrix} 0 & 0 & -1 & 1 & 0 & 0 & 1 & -1 \\ 0 & 0 & 1 & -1 & 0 & 0 & -1 & 1 \\ -1 & 1 & 0 & 0 & 1 & -1 & 0 & 0 \\ 1 & -1 & 0 & 0 & -1 & 1 & 0 & 0 \\ 0 & 0 & 1 & -1 & 1 & -1 & 0 & 0 \\ 0 & 0 & -1 & 1 & -1 & 1 & 0 & 0 \\ 1 & -1 & 0 & 0 & 0 & 0 & 1 & -1 \\ -1 & 1 & 0 & 0 & 0 & 0 & -1 & 1 \end{bmatrix}$</td>
</tr>
<tr>
<td>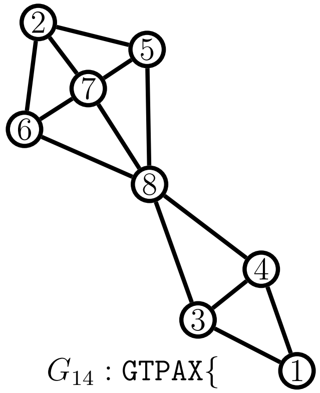<br>$G_{14}$ : GTPAX{</td>
<td>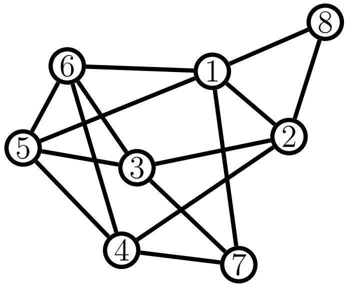<br>$\overline{G}_{14}$ : Gim|e?</td>
<td>$\begin{bmatrix} 0 & 0 & 1 & 2 & 0 & 0 & 0 & 0 \\ 0 & 0 & 0 & 0 & 2 & 2 & 1 & 0 \\ 1 & 0 & 1 & 1 & 0 & 0 & 0 & 1 \\ 2 & 0 & 1 & 0 & 0 & 0 & 0 & 2 \\ 0 & 2 & 0 & 0 & 0 & 0 & 1 & -2 \\ 0 & 2 & 0 & 0 & 0 & 0 & 1 & -2 \\ 0 & 1 & 0 & 0 & 1 & 1 & 1 & -1 \\ 0 & 0 & 1 & 2 & -2 & -2 & -1 & 0 \end{bmatrix}$</td>
<td>$\begin{bmatrix} -1 & 3 & 0 & 0 & 1 & 1 & -4 & 1 \\ 3 & -1 & -4 & 2 & 0 & 0 & 0 & -1 \\ 0 & -4 & 0 & 0 & -2 & -2 & 8 & 0 \\ 0 & 2 & 0 & 0 & 1 & 1 & -4 & 0 \\ 1 & 0 & -2 & 1 & 4 & -4 & 0 & 0 \\ 1 & 0 & -2 & 1 & -4 & 4 & 0 & 0 \\ -4 & 0 & 8 & -4 & 0 & 0 & 0 & 0 \\ 1 & -1 & 0 & 0 & 0 & 0 & 0 & -1 \end{bmatrix}$</td>
</tr>
<tr>
<td>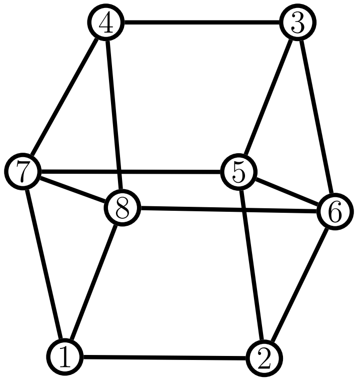<br>$G_{15}$ : G`Xksk</td>
<td>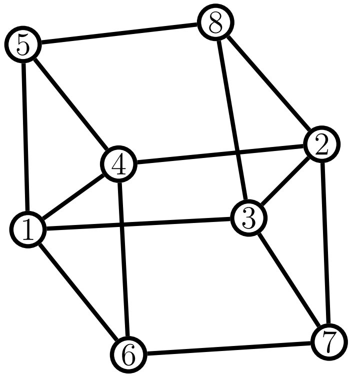<br>$\overline{G}_{15}$ : G]eRJO</td>
<td>$\begin{bmatrix} 2 & 2 & 0 & 0 & 0 & 0 & -2 & -2 \\ 2 & -2 & 0 & 0 & 1 & 2 & 0 & 0 \\ 0 & 0 & 2 & 2 & -1 & 2 & 0 & 0 \\ 0 & 0 & 2 & -2 & 0 & 0 & 2 & -2 \\ 0 & 1 & -1 & 0 & 0 & -1 & -1 & 0 \\ 0 & 2 & 2 & 0 & -1 & 0 & 0 & -2 \\ -2 & 0 & 0 & 2 & -1 & 0 & 0 & 2 \\ -2 & 0 & 0 & -2 & 0 & -2 & 2 & 0 \end{bmatrix}$</td>
<td>$\begin{bmatrix} 0 & 0 & -2 & -2 & -4 & 2 & 0 & 0 \\ 0 & 0 & -2 & 2 & 0 & 0 & 2 & -2 \\ -2 & -2 & 0 & 0 & 0 & 0 & -2 & -2 \\ -2 & 2 & 0 & 0 & 4 & 2 & 0 & 0 \\ -4 & 0 & 0 & 4 & 8 & 0 & 0 & -4 \\ 2 & 0 & 0 & 2 & 0 & -2 & 2 & 0 \\ 0 & 2 & -2 & 0 & 0 & 2 & 2 & 0 \\ 0 & -2 & -2 & 0 & -4 & 0 & 0 & -2 \end{bmatrix}$</td>
</tr>
</table>

| | | | |
|---|---|---|---|
| 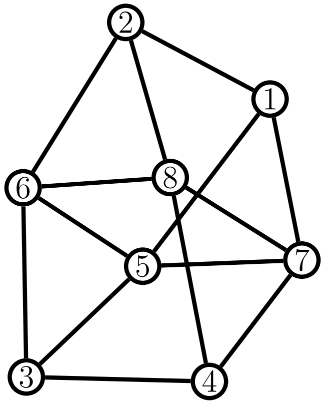 $G_{16}$ : G`hkqk | 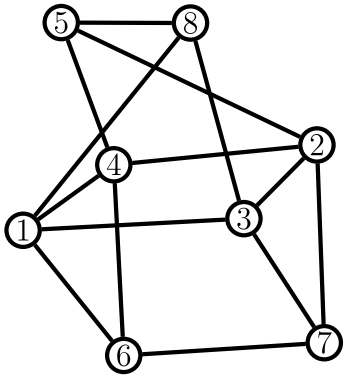 $\overline{G}_{16}$ : G]URLO | $\begin{bmatrix} 2 & 1 & 0 & 0 & -2 & 0 & -2 & 0 \\ 1 & 2 & 0 & 0 & 0 & -2 & 0 & 2 \\ 0 & 0 & -8 & -4 & 4 & 4 & 0 & 0 \\ 0 & 0 & -4 & -8 & 0 & 0 & 4 & -4 \\ -2 & 0 & 4 & 0 & 0 & -4 & 4 & 0 \\ 0 & -2 & 4 & 0 & -4 & 0 & 0 & -4 \\ -2 & 0 & 0 & 4 & 4 & 0 & 0 & 4 \\ 0 & 2 & 0 & -4 & 0 & -4 & 4 & 0 \end{bmatrix}$ | $\begin{bmatrix} 0 & 0 & 2 & -2 & 0 & 2 & 0 & 2 \\ 0 & 0 & -2 & 2 & -2 & 0 & 2 & 0 \\ 2 & -2 & 0 & 0 & 0 & 0 & 1 & 1 \\ -2 & 2 & 0 & 0 & -1 & 1 & 0 & 0 \\ 0 & -2 & 0 & -1 & -1 & 0 & 0 & 2 \\ 2 & 0 & 0 & 1 & 0 & 1 & 2 & 0 \\ 0 & 2 & 1 & 0 & 0 & 2 & 1 & 0 \\ 2 & 0 & 1 & 0 & 2 & 0 & 0 & -1 \end{bmatrix}$ |
| 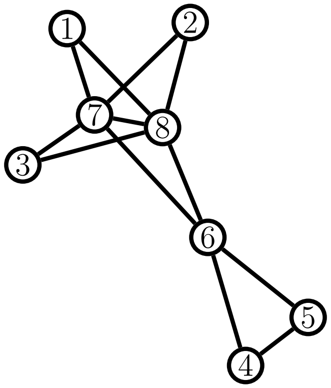 $G_{17}$ : G?C^NK | 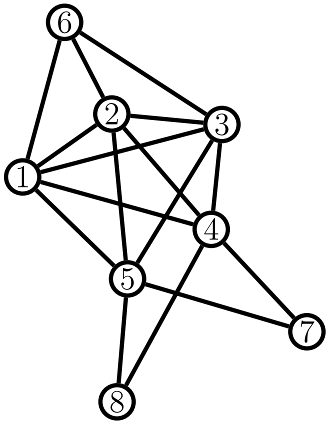 $\overline{G}_{17}$ : G∼z_oo | $\begin{bmatrix} 0 & 0 & 0 & 0 & 0 & 0 & 1 & 1 \\ 0 & 0 & 0 & 0 & 0 & 0 & 1 & 1 \\ 0 & 0 & 0 & 0 & 0 & 0 & 1 & 1 \\ 0 & 0 & 0 & 3 & 3 & -3 & 0 & 0 \\ 0 & 0 & 0 & 3 & 3 & -3 & 0 & 0 \\ 0 & 0 & 0 & -3 & -3 & 3 & -2 & -2 \\ 1 & 1 & 1 & 0 & 0 & -2 & 2 & 2 \\ 1 & 1 & 1 & 0 & 0 & -2 & 2 & 2 \end{bmatrix}$ | $\begin{bmatrix} -2 & -2 & 2 & -2 & 1 & -1 & 0 & 0 \\ -2 & -1 & 1 & 1 & -2 & -1 & 0 & 0 \\ 2 & 1 & 1 & 1 & 1 & 2 & 0 & 0 \\ -2 & 1 & 1 & 0 & 0 & 0 & 2 & -2 \\ 1 & -2 & 1 & 0 & 0 & 0 & -2 & 2 \\ -1 & -1 & 2 & 0 & 0 & 0 & 0 & 0 \\ 0 & 0 & 0 & 2 & -2 & 0 & 0 & 0 \\ 0 & 0 & 0 & -2 & 2 & 0 & 0 & 0 \end{bmatrix}$ |
| 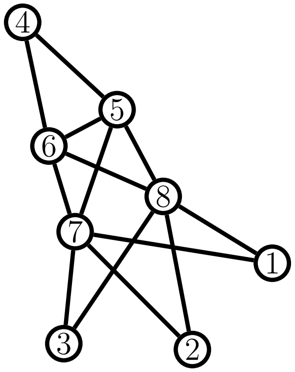 $G_{18}$ : G?C^^W | 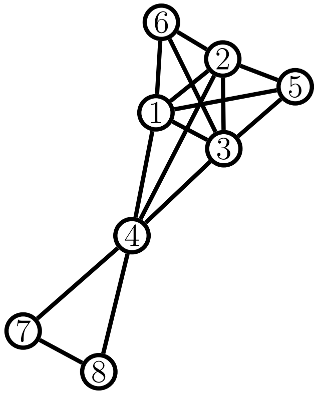 $\overline{G}_{18}$ : G∼z__c | $\begin{bmatrix} 0 & 0 & 0 & 0 & 0 & 0 & -2 & 1 \\ 0 & 0 & 0 & 0 & 0 & 0 & 2 & -1 \\ 0 & 0 & 0 & 0 & 0 & 0 & -2 & 1 \\ 0 & 0 & 0 & 0 & -1 & 1 & 0 & 0 \\ 0 & 0 & 0 & -1 & -2 & 1 & -2 & -1 \\ 0 & 0 & 0 & 1 & 1 & 0 & 2 & 1 \\ -2 & 2 & -2 & 0 & -2 & 2 & 0 & 0 \\ 1 & -1 & 1 & 0 & -1 & 1 & 0 & 0 \end{bmatrix}$ | $\begin{bmatrix} 4 & 2 & -2 & -6 & 6 & 6 & 0 & 0 \\ 2 & 8 & 6 & -10 & 10 & 10 & 0 & 0 \\ -2 & 6 & 8 & -4 & 4 & 4 & 0 & 0 \\ -6 & -10 & -4 & -48 & 0 & 0 & 12 & 24 \\ 6 & 10 & 4 & 0 & 0 & 0 & 0 & 0 \\ 6 & 10 & 4 & 0 & 0 & 0 & 0 & 0 \\ 0 & 0 & 0 & 12 & 0 & 0 & -3 & -6 \\ 0 & 0 & 0 & 24 & 0 & 0 & -6 & -12 \end{bmatrix}$ |

| | | | |
|---|---|---|---|
| 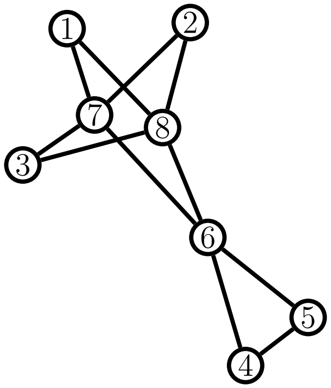 $G_{19}$ : G?C^NG | 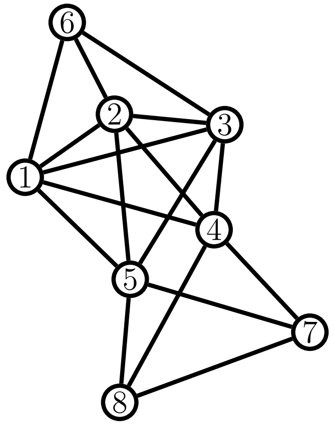 $\overline{G}_{19}$ : G∼z_os | $\begin{bmatrix} 0 & 0 & 0 & 0 & 0 & 0 & -1 & 1 \\ 0 & 0 & 0 & 0 & 0 & 0 & 1 & -1 \\ 0 & 0 & 0 & 0 & 0 & 0 & 2 & -2 \\ 0 & 0 & 0 & -1 & -1 & 1 & 0 & 0 \\ 0 & 0 & 0 & -1 & -1 & 1 & 0 & 0 \\ 0 & 0 & 0 & 1 & 1 & -1 & 1 & -1 \\ -1 & 1 & 2 & 0 & 0 & 1 & 0 & 0 \\ 1 & -1 & -2 & 0 & 0 & -1 & 0 & 0 \end{bmatrix}$ | $\begin{bmatrix} 5 & 2 & -2 & 14 & -7 & 7 & 0 & 0 \\ 2 & -13 & 5 & 4 & 1 & 5 & 0 & 0 \\ -2 & 5 & -4 & 5 & -4 & 1 & 0 & 0 \\ 14 & 4 & 5 & 0 & 0 & 0 & 4 & 4 \\ -7 & 1 & -4 & 0 & 0 & 0 & -4 & -4 \\ 7 & 5 & 1 & 0 & 0 & 0 & 0 & 0 \\ 0 & 0 & 0 & 4 & -4 & 0 & -5 & -5 \\ 0 & 0 & 0 & 4 & -4 & 0 & -5 & -5 \end{bmatrix}$ |
| 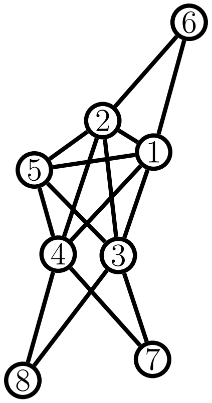 $G_{20}$ : G}∼@`_ | 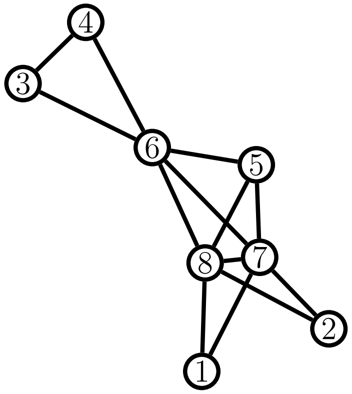 $\overline{G}_{20}$ : G@?}][ | $\begin{bmatrix} 0 & 1 & 1 & 2 & -1 & -2 & 0 & 0 \\ 1 & -2 & 2 & 1 & 1 & 2 & 0 & 0 \\ 1 & 2 & 0 & 0 & -1 & 0 & -2 & 1 \\ 2 & 1 & 0 & 0 & -1 & 0 & -2 & 1 \\ -1 & 1 & -1 & -1 & 0 & 0 & 0 & 0 \\ -2 & 2 & 0 & 0 & 0 & 0 & 0 & 0 \\ 0 & 0 & -2 & -2 & 0 & 0 & 0 & 0 \\ 0 & 0 & 1 & 1 & 0 & 0 & 0 & 0 \end{bmatrix}$ | $\begin{bmatrix} 0 & 0 & 0 & 0 & 0 & 0 & 5 & 10 \\ 0 & 0 & 0 & 0 & 0 & 0 & 5 & 10 \\ 0 & 0 & -10 & 10 & 0 & 5 & 0 & 0 \\ 0 & 0 & 10 & -10 & 0 & -5 & 0 & 0 \\ 0 & 0 & 0 & 0 & 10 & -5 & -3 & 4 \\ 0 & 0 & 5 & -5 & -5 & 0 & 4 & 3 \\ 5 & 5 & 0 & 0 & -3 & 4 & 8 & -2 \\ 10 & 10 & 0 & 0 & 4 & 3 & -2 & -30 \end{bmatrix}$ |

| | | | |
|---|---|---|---|
| 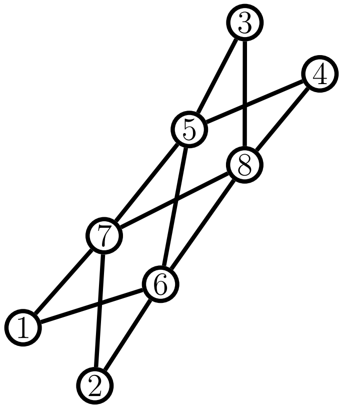<br>$G_{21}$ : G?NMPk | 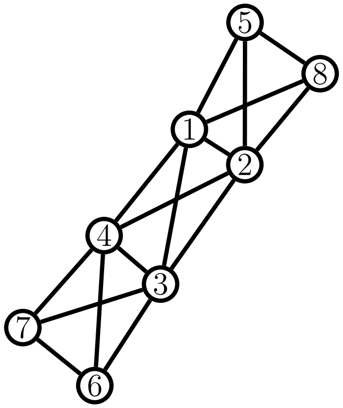<br>$\overline{G}_{21}$ : G~opmO | $\begin{bmatrix} 0 & 0 & 0 & 0 & 0 & -1 & 1 & 0 \\ 0 & 0 & 0 & 0 & 0 & -2 & 2 & 0 \\ 0 & 0 & 0 & 0 & 2 & 0 & 0 & 2 \\ 0 & 0 & 0 & 0 & 1 & 0 & 0 & 1 \\ 0 & 0 & 2 & 1 & 0 & 1 & -1 & 0 \\ -1 & -2 & 0 & 0 & 1 & 0 & 0 & 1 \\ 1 & 2 & 0 & 0 & -1 & 0 & 0 & -1 \\ 0 & 0 & 2 & 1 & 0 & 1 & -1 & 0 \end{bmatrix}$ | $\begin{bmatrix} 4 & -2 & 4 & -8 & -2 & 0 & 0 & 2 \\ -2 & 1 & -2 & 4 & 1 & 0 & 0 & -1 \\ 4 & -2 & -2 & 4 & 0 & -2 & -2 & 0 \\ -8 & 4 & 4 & -8 & 0 & 4 & 4 & 0 \\ -2 & 1 & 0 & 0 & -1 & 0 & 0 & 1 \\ 0 & 0 & -2 & 4 & 0 & 1 & 1 & 0 \\ 0 & 0 & -2 & 4 & 0 & 1 & 1 & 0 \\ 2 & -1 & 0 & 0 & 1 & 0 & 0 & -1 \end{bmatrix}$ |
| 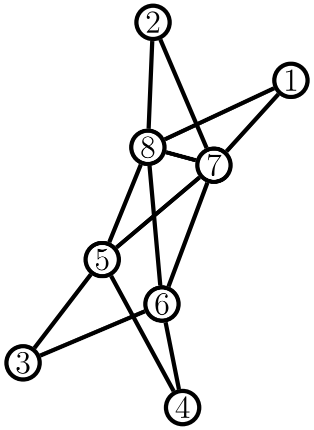<br>$G_{22}$ : G?Ku][ | 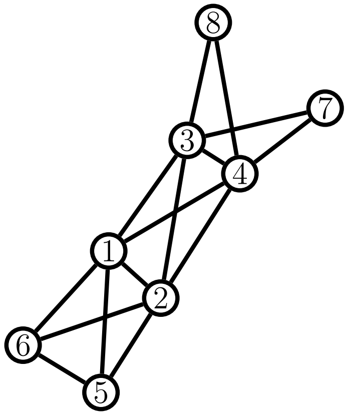<br>$\overline{G}_{22}$ : G~rH`_ | $\begin{bmatrix} 0 & 0 & 0 & 0 & 0 & 0 & -2 & 2 \\ 0 & 0 & 0 & 0 & 0 & 0 & -2 & 2 \\ 0 & 0 & 0 & 0 & 2 & 2 & 0 & 0 \\ 0 & 0 & 0 & 0 & 1 & 1 & 0 & 0 \\ 0 & 0 & 2 & 1 & 0 & 0 & 1 & -2 \\ 0 & 0 & 2 & 1 & 0 & 0 & -2 & 1 \\ -2 & -2 & 0 & 0 & 1 & -2 & 1 & -1 \\ 2 & 2 & 0 & 0 & -2 & 1 & -1 & 1 \end{bmatrix}$ | $\begin{bmatrix} 5.5 & 2 & 5 & -10 & 5 & -5 & 0 & 0 \\ 2 & -14 & -5 & 10 & -8 & 8 & 0 & 0 \\ 5 & -5 & -2 & 8 & 0 & 0 & 4 & 4 \\ -10 & 10 & 8 & -24 & 0 & 0 & -8 & -8 \\ 5 & -8 & 0 & 0 & -2 & 2 & 0 & 0 \\ -5 & 8 & 0 & 0 & 2 & -2 & 0 & 0 \\ 0 & 0 & 4 & -8 & 0 & 0 & 0 & 0 \\ 0 & 0 & 4 & -8 & 0 & 0 & 0 & 0 \end{bmatrix}$ |
| 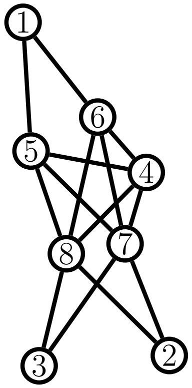<br>$G_{23}$ : G?eRzw | 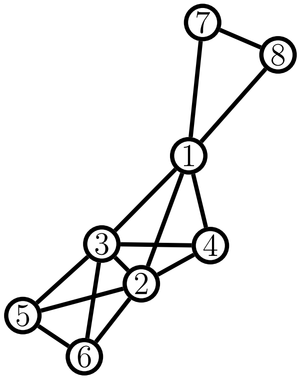<br>$\overline{G}_{23}$ : G~XkCC | $\begin{bmatrix} 0 & 0 & 0 & 0 & 2 & 2 & 0 & 0 \\ 0 & 0 & 0 & 0 & 0 & 0 & 2 & -2 \\ 0 & 0 & 0 & 0 & 0 & 0 & 1 & -1 \\ 0 & 0 & 0 & 0 & 2 & 2 & 2 & -2 \\ 2 & 0 & 0 & 2 & 0 & 0 & -1 & -1 \\ 2 & 0 & 0 & 2 & 0 & 0 & -1 & -1 \\ 0 & 2 & 1 & 2 & -1 & -1 & 0 & 0 \\ 0 & -2 & -1 & -2 & -1 & -1 & 0 & 0 \end{bmatrix}$ | $\begin{bmatrix} 7 & -4 & 2 & 3 & 0 & 0 & 10 & 10 \\ -4 & -7 & 6 & 4 & -2 & 2 & 0 & 0 \\ 2 & 6 & -8 & -2 & 4 & -4 & 0 & 0 \\ 3 & 4 & -2 & -3 & 0 & 0 & 0 & 0 \\ 0 & -2 & 4 & 0 & -2 & 2 & 0 & 0 \\ 0 & 2 & -4 & 0 & 2 & -2 & 0 & 0 \\ 10 & 0 & 0 & 0 & 0 & 0 & 10 & 10 \\ 10 & 0 & 0 & 0 & 0 & 0 & 10 & 10 \end{bmatrix}$ |

| | | | |
|---|---|---|---|
| 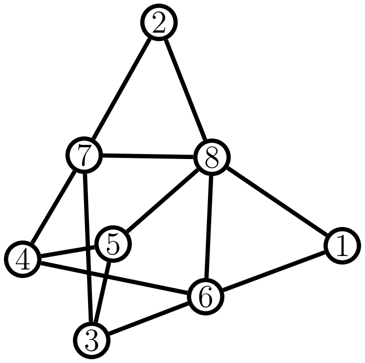 $G_{24}$ : G?Mre[ | 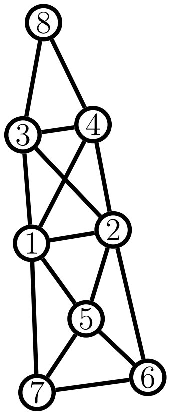 $\overline{G}_{24}$ : G~pKX_ | $\begin{bmatrix} -1 & 0 & 0 & 0 & 0 & 1 & 0 & -1 \\ 0 & -1 & 0 & 0 & 0 & 0 & -1 & 1 \\ 0 & 0 & 0 & 0 & 2 & 1 & 1 & 0 \\ 0 & 0 & 0 & 0 & 2 & 1 & 1 & 0 \\ 0 & 0 & 2 & 2 & 0 & 0 & 0 & 2 \\ 1 & 0 & 1 & 1 & 0 & -1 & 0 & 2 \\ 0 & -1 & 1 & 1 & 0 & 0 & -1 & 2 \\ -1 & 1 & 0 & 0 & 2 & 2 & 2 & -2 \end{bmatrix}$ | $\begin{bmatrix} 0 & 6 & -8 & 8 & 3 & 0 & -6 & 0 \\ 6 & 0 & 8 & -8 & -3 & 6 & 0 & 0 \\ -8 & 8 & 0 & -8 & 0 & 0 & 0 & 8 \\ 8 & -8 & -8 & 16 & 0 & 0 & 0 & -8 \\ 3 & -3 & 0 & 0 & -3 & 3 & 3 & 0 \\ 0 & 6 & 0 & 0 & 3 & 0 & -6 & 0 \\ -6 & 0 & 0 & 0 & 3 & -6 & 0 & 0 \\ 0 & 0 & 8 & -8 & 0 & 0 & 0 & 0 \end{bmatrix}$ |
| 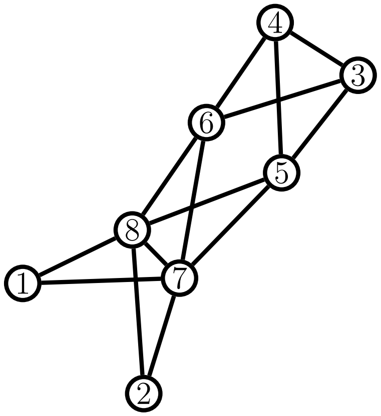 $G_{25}$ : G@Ku][ | 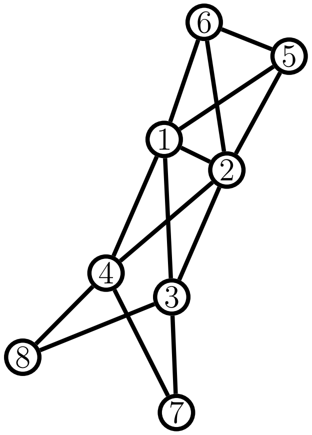 $\overline{G}_{25}$ : G}rH`_ | $\begin{bmatrix} 0 & 0 & 0 & 0 & 0 & 0 & 4 & 4 \\ 0 & 0 & 0 & 0 & 0 & 0 & 4 & 4 \\ 0 & 0 & 5 & 5 & 4 & 4 & 0 & 0 \\ 0 & 0 & 5 & 5 & 4 & 4 & 0 & 0 \\ 0 & 0 & 4 & 4 & 0 & 0 & 2 & 2 \\ 0 & 0 & 4 & 4 & 0 & 0 & -2 & -2 \\ 4 & 4 & 0 & 0 & 2 & -2 & -3 & -3 \\ 4 & 4 & 0 & 0 & 2 & -2 & -3 & -3 \end{bmatrix}$ | $\begin{bmatrix} 1 & 1 & 2 & -2 & -2 & 2 & 0 & 0 \\ 1 & -2 & -2 & 2 & 1 & -1 & 0 & 0 \\ 2 & -2 & 0 & 0 & 0 & 0 & -2 & 2 \\ -2 & 2 & 0 & 0 & 0 & 0 & 2 & -2 \\ -2 & 1 & 0 & 0 & 1 & -1 & 0 & 0 \\ 2 & -1 & 0 & 0 & -1 & 1 & 0 & 0 \\ 0 & 0 & -2 & 2 & 0 & 0 & 0 & 0 \\ 0 & 0 & 2 & -2 & 0 & 0 & 0 & 0 \end{bmatrix}$ |

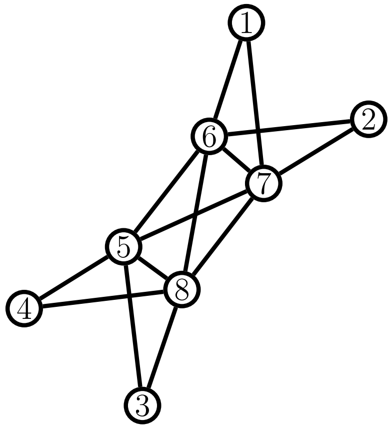

$G_{26}$ : `G?NMX{`

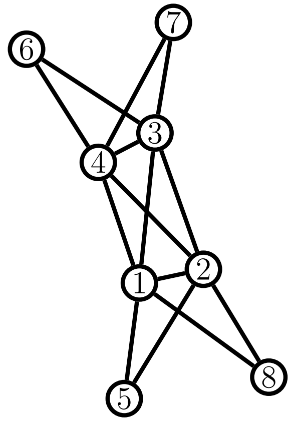

$\overline{G}_{26}$ : `G~ope?`

$$\begin{bmatrix} 0 & 0 & 0 & 0 & 0 & 2 & 2 & 0 \\ 0 & 0 & 0 & 0 & 0 & 2 & 2 & 0 \\ 0 & 0 & 0 & 0 & -1 & 0 & 0 & -1 \\ 0 & 0 & 0 & 0 & -1 & 0 & 0 & -1 \\ 0 & 0 & -1 & -1 & -2 & 2 & 2 & -1 \\ 2 & 2 & 0 & 0 & 2 & 2 & 2 & -2 \\ 2 & 2 & 0 & 0 & 2 & 2 & 2 & -2 \\ 0 & 0 & -1 & -1 & -1 & -2 & -2 & 0 \end{bmatrix}$$

$$\begin{bmatrix} 9 & 1 & 4 & 1 & -5 & 0 & 0 & 5 \\ 1 & -11 & -4 & -1 & 5 & 0 & 0 & -5 \\ 4 & -4 & 4 & -4 & 0 & 5 & -5 & 0 \\ 1 & -1 & -4 & 4 & 0 & -5 & 5 & 0 \\ -5 & 5 & 0 & 0 & 0 & 0 & 0 & 0 \\ 0 & 0 & 5 & -5 & 0 & 0 & 0 & 0 \\ 0 & 0 & -5 & 5 & 0 & 0 & 0 & 0 \\ 5 & -5 & 0 & 0 & 0 & 0 & 0 & 0 \end{bmatrix}$$

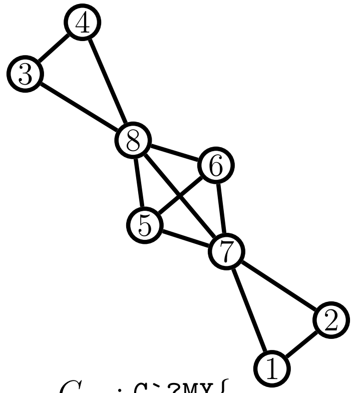

$G_{27}$ : ``G`?MX{``

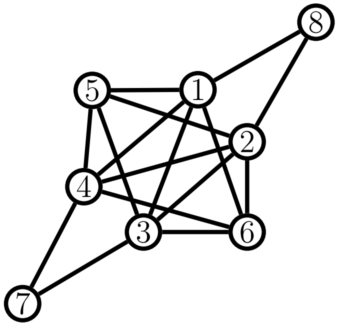

$\overline{G}_{27}$ : `G]~pe?`

$$\begin{bmatrix} 6 & 6 & 0 & 0 & 0 & 0 & 6 & 0 \\ 6 & 6 & 0 & 0 & 0 & 0 & 6 & 0 \\ 0 & 0 & 8 & -8 & 0 & 0 & 0 & -24 \\ 0 & 0 & -8 & 8 & 0 & 0 & 0 & 24 \\ 0 & 0 & 0 & 0 & -84 & -18 & 48 & 48 \\ 0 & 0 & 0 & 0 & -18 & -3 & 12 & 12 \\ 6 & 6 & 0 & 0 & 48 & 12 & -18 & -24 \\ 0 & 0 & -24 & 24 & 48 & 12 & -24 & 48 \end{bmatrix}$$

$$\begin{bmatrix} 0 & 0 & -2 & 1 & -1 & 2 & 0 & -1 \\ 0 & 0 & 1 & -2 & 1 & -2 & 0 & 1 \\ -2 & 1 & 0 & 0 & 1 & -2 & 1 & 0 \\ 1 & -2 & 0 & 0 & 1 & -2 & 1 & 0 \\ -1 & 1 & 1 & 1 & 0 & 0 & 0 & 0 \\ 2 & -2 & -2 & -2 & 0 & 0 & 0 & 0 \\ 0 & 0 & 1 & 1 & 0 & 0 & 0 & 0 \\ -1 & 1 & 0 & 0 & 0 & 0 & 0 & 0 \end{bmatrix}$$

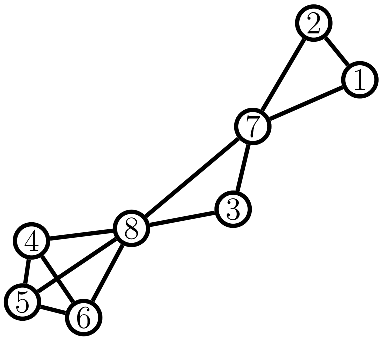

$G_{28}$ : `G_C^@{`

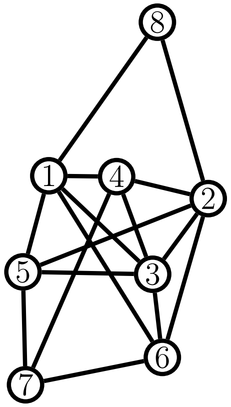

$\overline{G}_{28}$ : `G^z_}?`

$$\begin{bmatrix} 3 & 3 & 0 & 0 & 0 & 0 & -3 & 0 \\ 3 & 3 & 0 & 0 & 0 & 0 & -3 & 0 \\ 0 & 0 & -3 & 0 & 0 & 0 & 6 & 6 \\ 0 & 0 & 0 & 10 & 2 & 12 & 0 & 6 \\ 0 & 0 & 0 & 2 & -1 & 1 & 0 & -3 \\ 0 & 0 & 0 & 12 & 1 & 13 & 0 & 3 \\ -3 & -3 & 6 & 0 & 0 & 0 & -9 & -12 \\ 0 & 0 & 6 & 6 & -3 & 3 & -12 & -21 \end{bmatrix}$$

$$\begin{bmatrix} 0 & 0 & 2 & 2 & -1 & -2 & 0 & 1 \\ 0 & 0 & -2 & -1 & 2 & 1 & 0 & -1 \\ 2 & -2 & 0 & 2 & 2 & -2 & 0 & 0 \\ 2 & -1 & 2 & 0 & 0 & 0 & 1 & 0 \\ -1 & 2 & 2 & 0 & 0 & 0 & 1 & 0 \\ -2 & 1 & -2 & 0 & 0 & 0 & -1 & 0 \\ 0 & 0 & 0 & 1 & 1 & -1 & 0 & 0 \\ 1 & -1 & 0 & 0 & 0 & 0 & 0 & 0 \end{bmatrix}$$

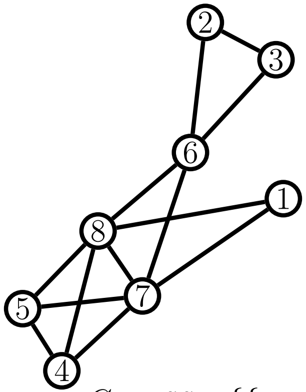

$G_{29}$ : GGDc{{

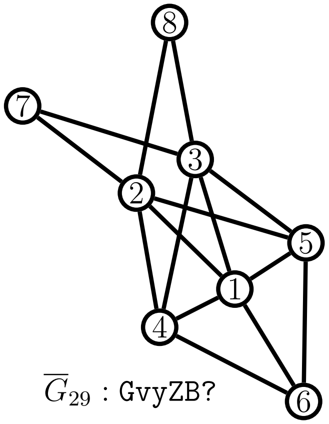

$\overline{G}_{29}$ : GvyZB?

$$\begin{bmatrix} 0 & 0 & 0 & 0 & 0 & 0 & 4 & 4 \\ 0 & -1 & -1 & 0 & 0 & -2 & 0 & 0 \\ 0 & -1 & -1 & 0 & 0 & -2 & 0 & 0 \\ 0 & 0 & 0 & -4 & 4 & 0 & 4 & 4 \\ 0 & 0 & 0 & 4 & -4 & 0 & -2 & -2 \\ 0 & -2 & -2 & 0 & 0 & -4 & 2 & 2 \\ 4 & 0 & 0 & 4 & -2 & 2 & 3 & 3 \\ 4 & 0 & 0 & 4 & -2 & 2 & 3 & 3 \end{bmatrix}$$

$$\begin{bmatrix} 1 & 1 & 1 & -1 & -1 & -1 & 0 & 0 \\ 1 & 0 & 0 & -2 & -2 & 0 & 1 & -1 \\ 1 & 0 & 0 & -2 & -2 & 0 & -1 & 1 \\ -1 & -2 & -2 & 0 & 0 & 2 & 0 & 0 \\ -1 & -2 & -2 & 0 & 0 & 2 & 0 & 0 \\ -1 & 0 & 0 & 2 & 2 & 0 & 0 & 0 \\ 0 & 1 & -1 & 0 & 0 & 0 & 0 & 0 \\ 0 & -1 & 1 & 0 & 0 & 0 & 0 & 0 \end{bmatrix}$$

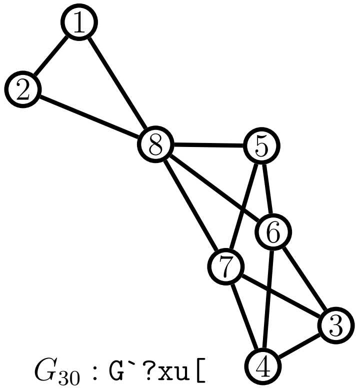

$G_{30}$ : G`?xu[

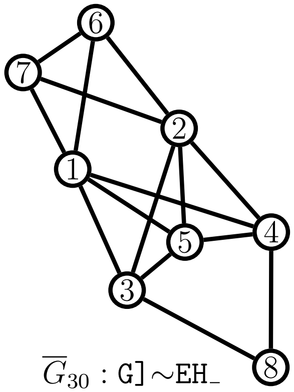

$\overline{G}_{30}$ : G]∼EH_

$$\begin{bmatrix} 18 & 18 & 0 & 0 & 0 & 0 & 0 & -9 \\ 18 & 18 & 0 & 0 & 0 & 0 & 0 & -9 \\ 0 & 0 & -5 & 5 & 0 & -15 & 15 & 0 \\ 0 & 0 & 5 & -5 & 0 & 15 & -15 & 0 \\ 0 & 0 & 0 & 0 & 45 & 45 & -45 & 45 \\ 0 & 0 & -15 & 15 & 45 & 0 & 0 & 45 \\ 0 & 0 & 15 & -15 & -45 & 0 & 0 & -45 \\ -9 & -9 & 0 & 0 & 45 & 45 & -45 & 49.5 \end{bmatrix}$$

$$\begin{bmatrix} 0 & 0 & -2 & 1 & -1 & 2 & 1 & 0 \\ 0 & 0 & 1 & -2 & 1 & -2 & -1 & 0 \\ -2 & 1 & 0 & 0 & 2 & 0 & 0 & -2 \\ 1 & -2 & 0 & 0 & 2 & 0 & 0 & -2 \\ -1 & 1 & 2 & 2 & 0 & 0 & 0 & 0 \\ 2 & -2 & 0 & 0 & 0 & 1 & 1 & 0 \\ 1 & -1 & 0 & 0 & 0 & 1 & 1 & 0 \\ 0 & 0 & -2 & -2 & 0 & 0 & 0 & 0 \end{bmatrix}$$

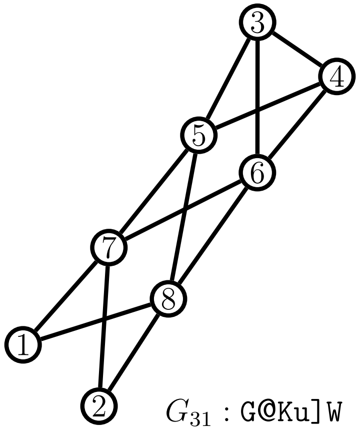

$G_{31}$ : G@Ku]W

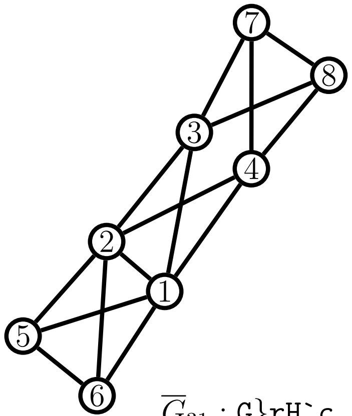

$\overline{G}_{31}$ : G}rH`c

$$\begin{bmatrix} 0 & 0 & 0 & 0 & 0 & 0 & 2 & -2 \\ 0 & 0 & 0 & 0 & 0 & 0 & 1 & -1 \\ 0 & 0 & -2 & 2 & -1 & -1 & 0 & 0 \\ 0 & 0 & 2 & -2 & 1 & 1 & 0 & 0 \\ 0 & 0 & -1 & 1 & 0 & 0 & -1 & 1 \\ 0 & 0 & -1 & 1 & 0 & 0 & -2 & 2 \\ 2 & 1 & 0 & 0 & -1 & -2 & 0 & 0 \\ -2 & -1 & 0 & 0 & 1 & 2 & 0 & 0 \end{bmatrix}$$

$$\begin{bmatrix} -1 & -4 & -4 & -4 & 6 & -6 & 0 & 0 \\ -4 & 12 & 8 & 8 & -4 & 4 & 0 & 0 \\ -4 & 8 & 0 & 0 & 0 & 0 & 4 & 4 \\ -4 & 8 & 0 & 0 & 0 & 0 & 4 & 4 \\ 6 & -4 & 0 & 0 & -8 & 8 & 0 & 0 \\ -6 & 4 & 0 & 0 & 8 & -8 & 0 & 0 \\ 0 & 0 & 4 & 4 & 0 & 0 & -4 & -4 \\ 0 & 0 & 4 & 4 & 0 & 0 & -4 & -4 \end{bmatrix}$$

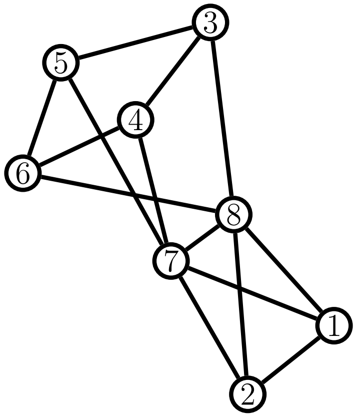

$G_{32}$ : G`G]vK

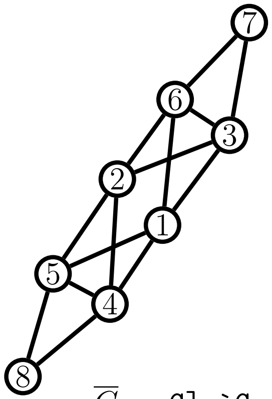

$\overline{G}_{32}$ : G]v`Go

$$\begin{bmatrix} 0 & 2 & 0 & 0 & 0 & 0 & 1 & 1 \\ 2 & 0 & 0 & 0 & 0 & 0 & 2 & -2 \\ 0 & 0 & 0 & 1 & 1 & 0 & 0 & -1 \\ 0 & 0 & 1 & 0 & 0 & 1 & -1 & 0 \\ 0 & 0 & 1 & 0 & 0 & 1 & -1 & 0 \\ 0 & 0 & 0 & 1 & 1 & 0 & 0 & -1 \\ 1 & 2 & 0 & -1 & -1 & 0 & 2 & 1 \\ 1 & -2 & -1 & 0 & 0 & -1 & 1 & -2 \end{bmatrix}$$

$$\begin{bmatrix} 0 & 0 & 2 & 4 & -4 & -2 & 0 & 0 \\ 0 & 0 & 1 & -2 & 2 & -1 & 0 & 0 \\ 2 & 1 & -6 & 0 & 0 & 4 & -2 & 0 \\ 4 & -2 & 0 & 2 & 2 & 0 & 0 & 4 \\ -4 & 2 & 0 & 2 & -6 & 0 & 0 & -4 \\ -2 & -1 & 4 & 0 & 0 & -2 & 2 & 0 \\ 0 & 0 & -2 & 0 & 0 & 2 & 0 & 0 \\ 0 & 0 & 0 & 4 & -4 & 0 & 0 & 0 \end{bmatrix}$$

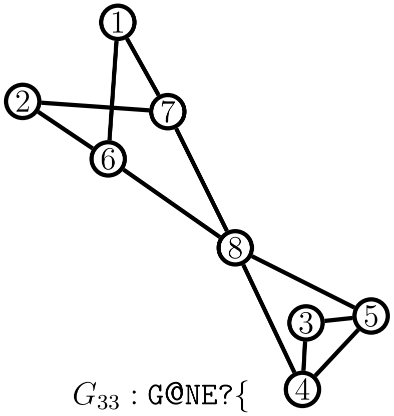

$G_{33}$ : G@NE?{

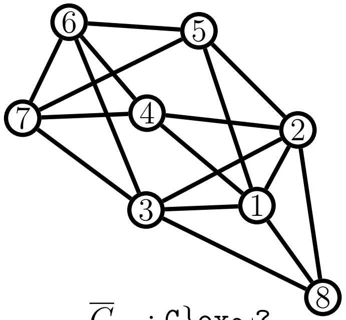

$\overline{G}_{33}$ : G}ox∼?

$$\begin{bmatrix} 0 & 0 & 0 & 0 & 0 & 2 & 2 & 0 \\ 0 & 0 & 0 & 0 & 0 & 1 & 1 & 0 \\ 0 & 0 & 0 & -1 & 1 & 0 & 0 & 0 \\ 0 & 0 & -1 & 0 & 1 & 0 & 0 & 1 \\ 0 & 0 & 1 & 1 & -2 & 0 & 0 & -1 \\ 2 & 1 & 0 & 0 & 0 & 0 & 0 & -2 \\ 2 & 1 & 0 & 0 & 0 & 0 & 0 & -2 \\ 0 & 0 & 0 & 1 & -1 & -2 & -2 & 0 \end{bmatrix}$$

$$\begin{bmatrix} 1 & 8 & 7 & 2 & 2 & 0 & 0 & 5 \\ 8 & 4 & 6 & -4 & -4 & 0 & 0 & 10 \\ 7 & 6 & 10 & 0 & 0 & 10 & -10 & 10 \\ 2 & -4 & 0 & 0 & 0 & 10 & -10 & 0 \\ 2 & -4 & 0 & 0 & 0 & 10 & -10 & 0 \\ 0 & 0 & 10 & 10 & 10 & -8 & 8 & 0 \\ 0 & 0 & -10 & -10 & -10 & 8 & -8 & 0 \\ 5 & 10 & 10 & 0 & 0 & 0 & 0 & 10 \end{bmatrix}$$

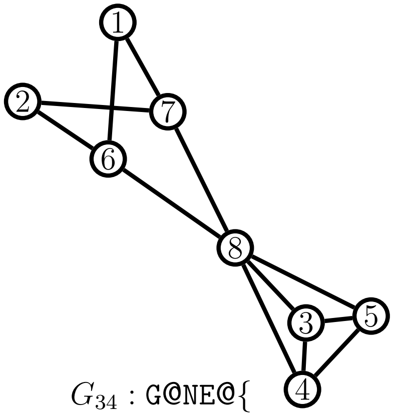

$G_{34}$ : G@NE@{

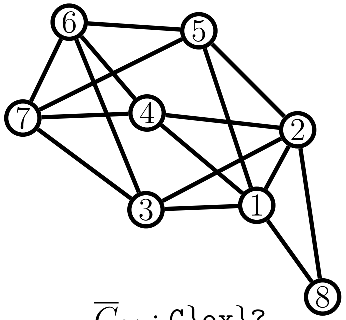

$\overline{G}_{34}$ : G}ox}?

$$\begin{bmatrix} 0 & 0 & 0 & 0 & 0 & 1 & 2 & 0 \\ 0 & 0 & 0 & 0 & 0 & 1 & 2 & 0 \\ 0 & 0 & 2 & 1 & 1 & 0 & 0 & 2 \\ 0 & 0 & 1 & 0 & 1 & 0 & 0 & 1 \\ 0 & 0 & 1 & 1 & 0 & 0 & 0 & 1 \\ 1 & 1 & 0 & 0 & 0 & 0 & 0 & -1 \\ 2 & 2 & 0 & 0 & 0 & 0 & 0 & -2 \\ 0 & 0 & 2 & 1 & 1 & -1 & -2 & 2 \end{bmatrix}$$

$$\begin{bmatrix} 0 & 4 & -8 & 4 & 4 & 0 & 0 & 4 \\ 4 & -8 & 8 & -4 & -4 & 0 & 0 & -4 \\ -8 & 8 & 0 & 0 & 0 & -4 & 2 & 0 \\ 4 & -4 & 0 & 0 & 0 & 4 & -2 & 0 \\ 4 & -4 & 0 & 0 & 0 & 4 & -2 & 0 \\ 0 & 0 & -4 & 4 & 4 & 12 & -6 & 0 \\ 0 & 0 & 2 & -2 & -2 & -6 & 3 & 0 \\ 4 & -4 & 0 & 0 & 0 & 0 & 0 & 0 \end{bmatrix}$$

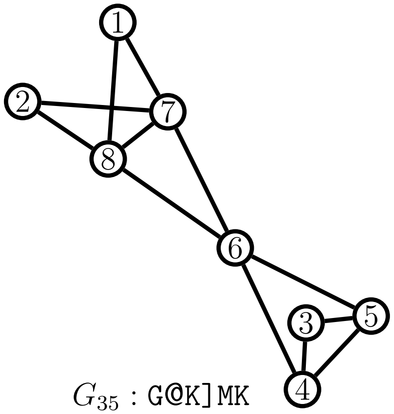


$G_{35}$ : `G@K]MK`

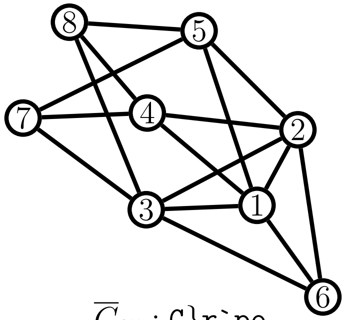


$\overline{G}_{35}$ : `G}r`po`

$$\begin{bmatrix} 0 & 0 & 0 & 0 & 0 & 0 & -1 & -1 \\ 0 & 0 & 0 & 0 & 0 & 0 & 1 & 1 \\ 0 & 0 & 0 & -1 & -1 & 0 & 0 & 0 \\ 0 & 0 & -1 & 2 & 1 & 1 & 0 & 0 \\ 0 & 0 & -1 & 1 & 0 & 1 & 0 & 0 \\ 0 & 0 & 0 & 1 & 1 & 0 & 2 & 2 \\ -1 & 1 & 0 & 0 & 0 & 2 & -2 & -1 \\ -1 & 1 & 0 & 0 & 0 & 2 & -1 & 0 \end{bmatrix}$$

$$\begin{bmatrix} 26 & 2 & 6 & -6 & 6 & 12 & 0 & 0 \\ 2 & -6 & -1 & -5 & 5 & 4 & 0 & 0 \\ 6 & -1 & 4 & 0 & 0 & 4 & 1 & -1 \\ -6 & -5 & 0 & 0 & 0 & 0 & 1 & -1 \\ 6 & 5 & 0 & 0 & 0 & 0 & -1 & 1 \\ 12 & 4 & 4 & 0 & 0 & 4 & 0 & 0 \\ 0 & 0 & 1 & 1 & -1 & 0 & 0 & 0 \\ 0 & 0 & -1 & -1 & 1 & 0 & 0 & 0 \end{bmatrix}$$

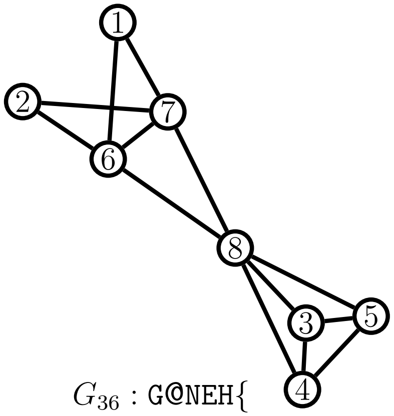


$G_{36}$ : `G@NEH{`

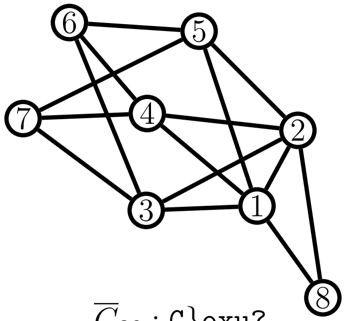


$\overline{G}_{36}$ : `G}oxu?`

$$\begin{bmatrix} 0 & 0 & 0 & 0 & 0 & -12 & -12 & 0 \\ 0 & 0 & 0 & 0 & 0 & 12 & 12 & 0 \\ 0 & 0 & -4 & -3 & -7 & 0 & 0 & -15 \\ 0 & 0 & -3 & 18 & 15 & 0 & 0 & 9 \\ 0 & 0 & -7 & 15 & 8 & 0 & 0 & -6 \\ -12 & 12 & 0 & 0 & 0 & 6 & 6 & 12 \\ -12 & 12 & 0 & 0 & 0 & 6 & 6 & 12 \\ 0 & 0 & -15 & 9 & -6 & 12 & 12 & -36 \end{bmatrix}$$

$$\begin{bmatrix} 2 & 1 & -1 & 1 & -2 & 0 & 0 & 1 \\ 1 & 0 & -1 & 1 & -2 & 0 & 0 & 1 \\ -1 & -1 & 0 & 0 & 0 & -2 & 2 & 0 \\ 1 & 1 & 0 & 0 & 0 & -2 & 2 & 0 \\ -2 & -2 & 0 & 0 & 0 & 2 & -2 & 0 \\ 0 & 0 & -2 & -2 & 2 & 0 & 0 & 0 \\ 0 & 0 & 2 & 2 & -2 & 0 & 0 & 0 \\ 1 & 1 & 0 & 0 & 0 & 0 & 0 & 0 \end{bmatrix}$$
